# Supplementary material for: MDIntrinsicDimension: Dimensionality-Based Analysis of Collective Motions in Macromolecules from Molecular Dynamics Trajectories
Source: arXiv:2511.13550 ancillary file (2026-02-27)
Supplement: Supplementary file 1 [file supp.pdf]

# Supplementary Data

## MDIntrinsicDimension: Dimensionality-Based Analysis of Collective Modes of Macromolecules from Molecular Dynamics Trajectories

Irene Cazzaniga<sup>1</sup>, Toni Giorgino<sup>1</sup>

<sup>1</sup>Istituto di Biofisica (IBF-CNR), Consiglio Nazionale delle Ricerche, Milano, Italy.

### 1 Supplementary Data for the Methods Section

| Estimator name                                   | Abbreviation | Type   | Reference |
|--------------------------------------------------|--------------|--------|-----------|
| Correlation (fractal) dimensionality             | CorrInt      | local  | [1]       |
| Dimensionality from angle and norm concentration | DANCo        | global | [2]       |
| Expected simplex skewness                        | ESS          | global | [3]       |
| Fisher separability                              | FisherS      | global | [4]       |
| Weighted average kNN distances                   | KNN          | local  | [5]       |
| Local principal component analysis               | lPCA         | local  | [6]       |
| Manifold-adaptive fractal dimension              | MADA         | local  | [7]       |
| Minimum neighbor distance–maximum likelihood     | MiND_ML      | global | [8]       |
| Maximum likelihood estimator                     | MLE          | local  | [9]       |
| Method of moments                                | MOM          | local  | [10]      |
| Tight localities estimator                       | TLE          | global | [11]      |
| Two-nearest neighbours                           | TwoNN        | global | [12]      |

Table S1: ID estimators supported by the `scikit-dimension` library (alphabetically ordered).

## 2 Supplementary Data for the Villin HP35 Case Study

| TS  | Key | Frames     | State    |
|-----|-----|------------|----------|
| 000 | u0  | 0–2000     | Unfolded |
| 001 | f0  | 0–2000     | Folded   |
| 001 | u1  | 5000–7000  | Unfolded |
| 004 | f1  | 8000–10000 | Folded   |
| 005 | u2  | 1700–3700  | Unfolded |
| 005 | f2  | 5000–7000  | Folded   |

Table S2: Subsections of the villin trajectories selected for analyses, split into three periods in the folded state and three in the unfolded state. *TS* is the trajectory segment, i.e. the dotted part in trajectory file names 2F4K-protein-0-....dcd from [13]; *Key* is the corresponding abbreviation used in the legends.

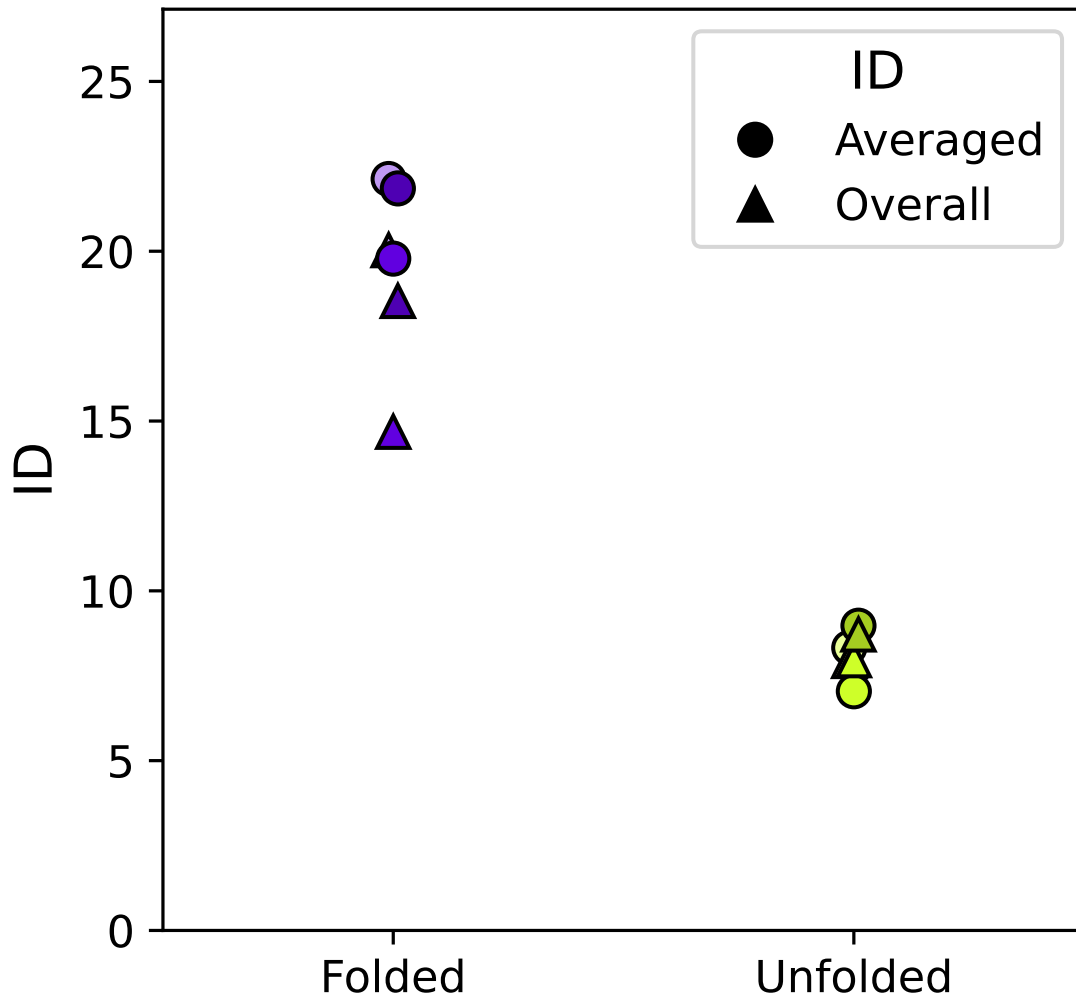

Figure S1: Averaged (circles) and overall (triangles) ID of the villin trajectories. In both cases,  $\phi$  and  $\psi$  dihedral angles were used as a projection.

### 3 Supplementary Data for the NTL9 Case Study

In the following, “NTL9” refers to the N-terminal Domain of Ribosomal Protein L9 (NTL9, PDB:2HBA(1-39)). Trajectories refer to DESRES-Trajectory NTL9-2-protein dataset from the D. E. Shaw Research fast-folding proteins [13]. If not stated otherwise, the estimator of choice is *TwoNN* [12], and the projections are computed from  $\phi$  and  $\psi$  Ramachandran angles.

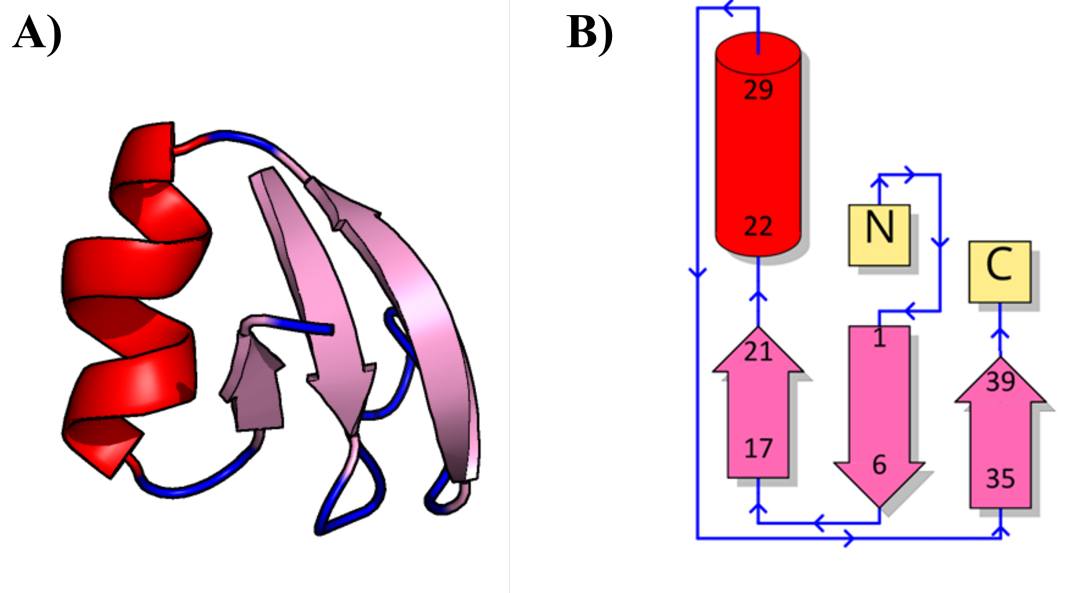

Figure S2: NTL9 (PDB 2HBA), 39-residue protein structure (A), colored by secondary structure and corresponding topology diagram (B).

| Traj | Key | Frames | State    |
|------|-----|--------|----------|
| 000  | u0  | 0–2000 | Unfolded |
| 050  | f0  | 0–2000 | Folded   |
| 080  | u1  | 0–2000 | Unfolded |
| 100  | f1  | 0–2000 | Folded   |
| 124  | u2  | 0–2000 | Unfolded |
| 194  | f2  | 0–2000 | Folded   |

Table S3: Subsections of the NTL9 trajectories selected for analyses, sliced into three periods in the folded state and three in the unfolded state. “Traj” correspond the trailing part of data files names NTL9-2-protein-....dcd and accompanying paper [13]; “Key” is the corresponding abbreviation used in the legends.

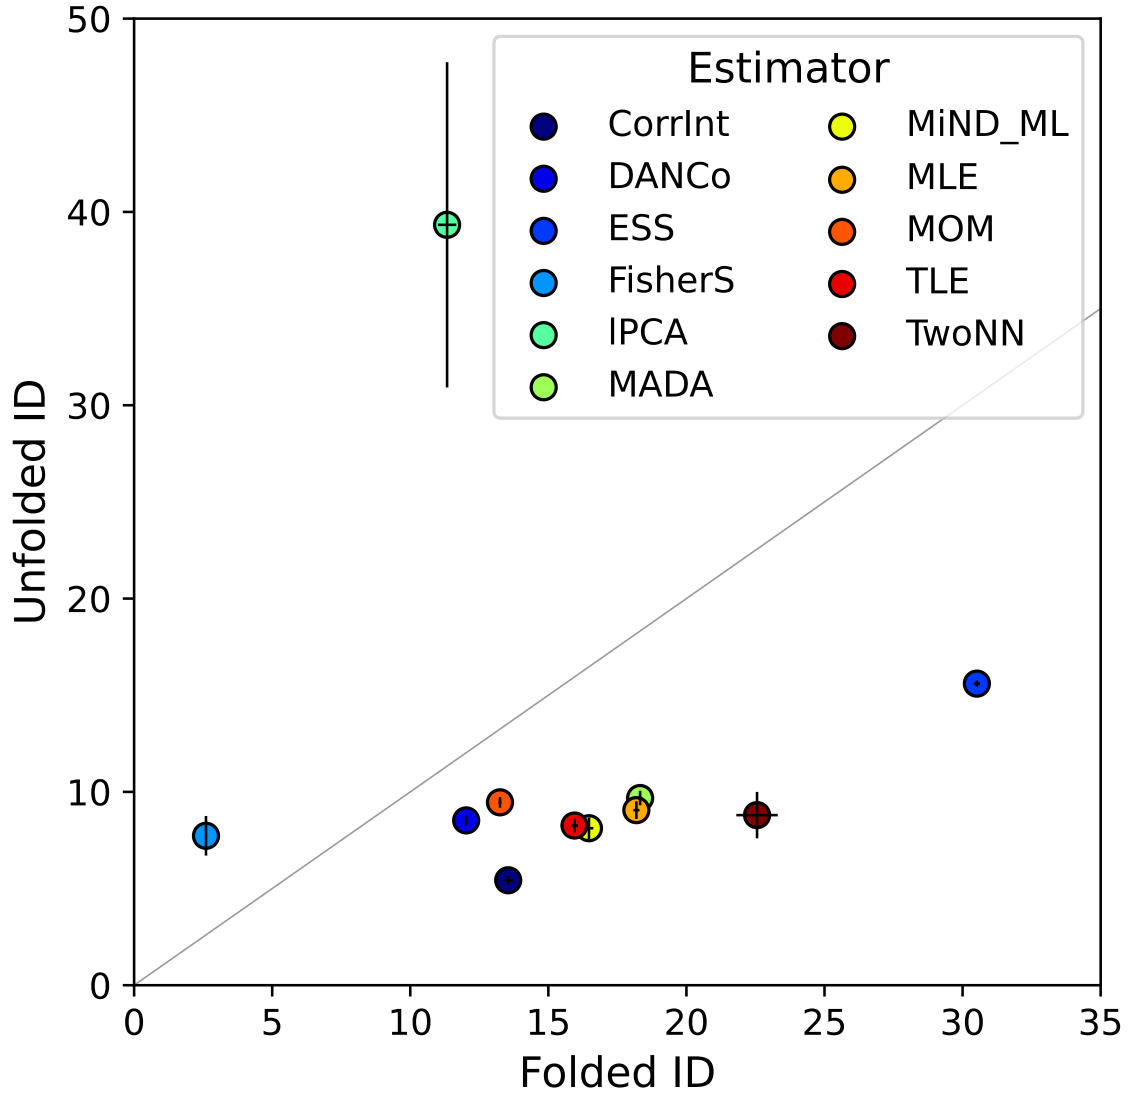

Figure S3: Folded–vs–unfolded ID of the NTL9 dynamic manifold, computed by the estimators available at `scikit-dimension` package. Each point represents the mean value of the folded states ( $x$  axis) and unfolded states ( $y$  axis). Error bars parallel to each axis indicate the standard deviation from the mean for the respective state.

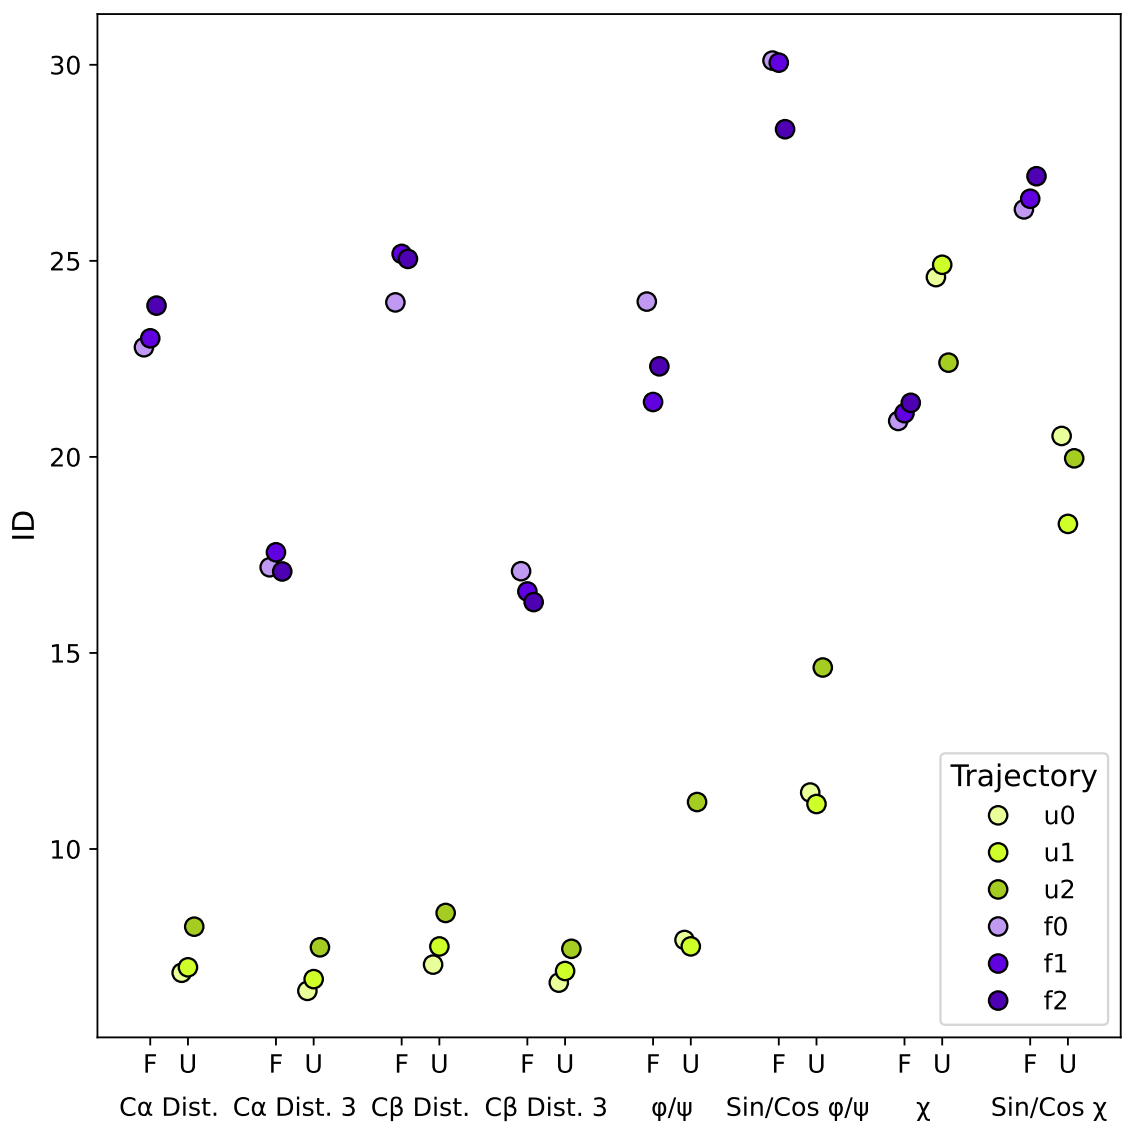

Figure S4: Differences in ID between folded (f) and unfolded (u) states on NTL9 under different projections. *Dist.*: pairwise distances between all carbon-carbon pairs; *Dist. 3*: pairwise distances every 3rd carbon;  $\phi, \psi$ : Ramachandran angles;  $\chi$ : sidechain dihedrals; *Sin/Cos*: trigonometric embedding of angles.

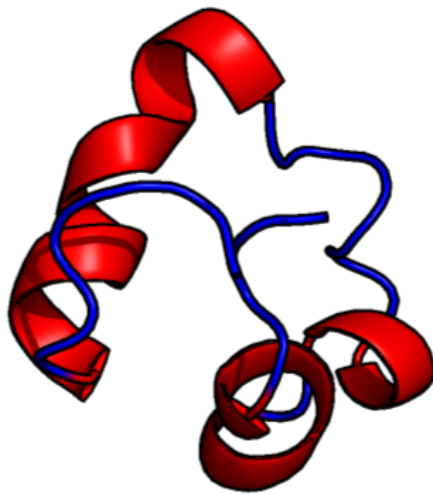

Figure S5: NTL9 transient folded structure found in trajectory `u2` at frame 1700.

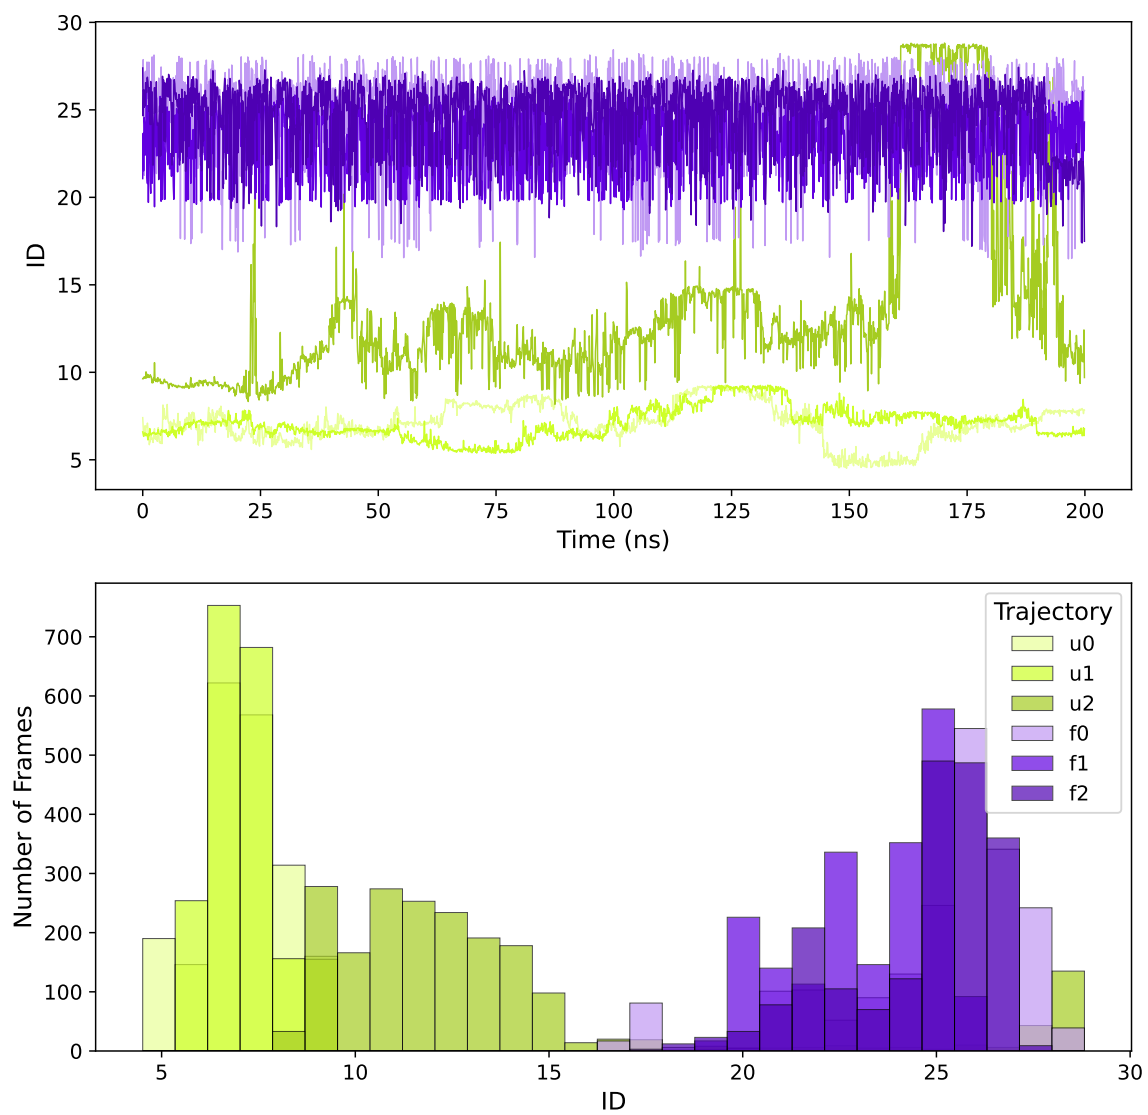

Figure S6: Instantaneous ID over time (top panel) and ID distribution frequency (bottom panel) along the trajectory. In violet, folded protein trajectories; in green, unfolded ones.

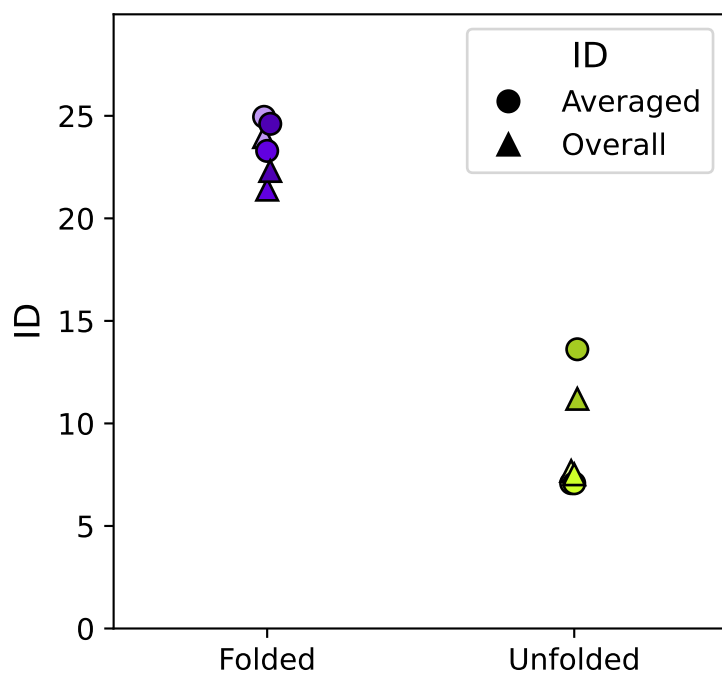

Figure S7: Averaged (circles) and overall (triangles) ID from individual trajectories.

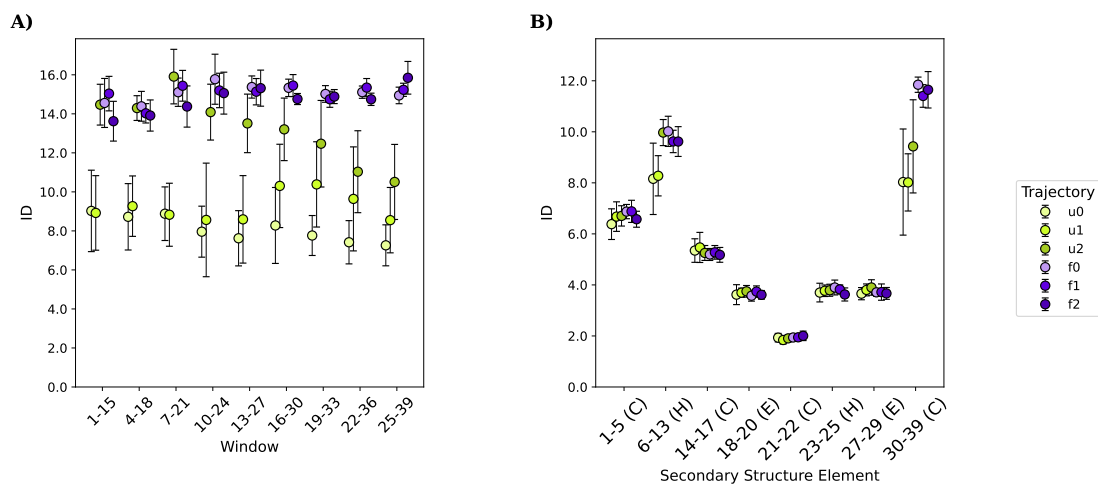

Figure S8: ID computed on structural local regions. (A) Sequence-wise ID computed with `section_id()` using a *window* of 15 and *stride* of 3. (B) Structure-wise ID computed with `secondary_structure_id()`, using a simplified DSSP.



## References

- [1] Grassberger P, Procaccia I. Measuring the strangeness of strange attractors. *Physica D: Nonlinear Phenomena*. 1983 Oct;9(1-2):189-208. Available from: <https://linkinghub.elsevier.com/retrieve/pii/0167278983902981>.
- [2] Ceruti C, Bassis S, Rozza A, Lombardi G, Casiraghi E, Campadelli P. DANCo: An intrinsic dimensionality estimator exploiting angle and norm concentration. *Pattern Recognition*. 2014 Aug;47(8):2569-81. Available from: <https://linkinghub.elsevier.com/retrieve/pii/S003132031400065X>.
- [3] Johnsson K, Sonesson C, Fontes M. Low Bias Local Intrinsic Dimension Estimation from Expected Simplex Skewness. *IEEE Transactions on Pattern Analysis and Machine Intelligence*. 2015 Jan;37(1):196-202. Available from: <http://ieeexplore.ieee.org/document/6866171/>.
- [4] Albergante L, Bac J, Zinovyev A. Estimating the effective dimension of large biological datasets using Fisher separability analysis. In: 2019 International Joint Conference on Neural Networks (IJCNN). Budapest, Hungary: IEEE; 2019. p. 1-8. Available from: <https://ieeexplore.ieee.org/document/8852450/>.
- [5] Carter KM, Raich R, Hero AO. On Local Intrinsic Dimension Estimation and Its Applications. *IEEE Transactions on Signal Processing*. 2010 Feb;58(2):650-63. Available from: <http://ieeexplore.ieee.org/document/5233815/>.
- [6] Fukunaga K, Olsen DR. An Algorithm for Finding Intrinsic Dimensionality of Data. *IEEE Transactions on Computers*. 1971 Feb;C-20(2):176-83. Conference Name: IEEE Transactions on Computers.
- [7] Farahmand AM, Szepesvári C, Audibert JY. Manifold-adaptive dimension estimation. In: Proceedings of the 24th international conference on Machine learning. Corvallis Oregon USA: ACM; 2007. p. 265-72. Available from: <https://dl.acm.org/doi/10.1145/1273496.1273530>.
- [8] Rozza A, Lombardi G, Ceruti C, Casiraghi E, Campadelli P. Novel high intrinsic dimensionality estimators. *Machine Learning*. 2012 Oct;89(1-2):37-65. Available from: <http://link.springer.com/10.1007/s10994-012-5294-7>.
- [9] Levina E, Bickel PJ. Maximum Likelihood Estimation of Intrinsic Dimension. In: Saul LK, Weiss Y, Bottou L, editors. *Advances in Neural Information Processing Systems 17*. MIT Press; 2005. p. 777-84. Available from: <http://papers.nips.cc/paper/2577-maximum-likelihood-estimation-of-intrinsic-dimension.pdf>.
- [10] Amsaleg L, Chelly O, Furon T, Girard S, Houle ME, Kawarabayashi Ki, et al. Extreme-value-theoretic estimation of local intrinsic dimensionality. *Data Mining and Knowledge Discovery*. 2018 Nov;32(6):1768-805. Available from: <http://link.springer.com/10.1007/s10618-018-0578-6>.
- [11] Amsaleg L, Chelly O, Houle ME, Kawarabayashi Ki, Radovanović M, Treeratnanajaru W. Intrinsic Dimensionality Estimation within Tight Localities: A Theoretical and Experimental Analysis. *arXiv*; 2022. ArXiv:2209.14475 [cs]. Available from: <http://arxiv.org/abs/2209.14475>.
- [12] Facco E, d'Errico M, Rodriguez A, Laio A. Estimating the intrinsic dimension of datasets by a minimal neighborhood information. *Scientific Reports*. 2017 Sep;7(1):12140. Available from: <https://www.nature.com/articles/s41598-017-11873-y>.
- [13] Lindorff-Larsen K, Piana S, Dror RO, Shaw DE. How Fast-Folding Proteins Fold. *Science*. 2011 Oct;334(6055):517-20. Available from: <https://www.science.org/doi/10.1126/science.1208351>.
